# Supplementary material for: On the Voting Time of the Deterministic Majority Process
Source: arXiv:1508.03519 source file (2015-08-14)
Supplement: Supplementary file 1 [file appendix-examples.tex]

\section{Examples}

\subsection{The Grid}

\begin{figure}[h]
\centering
\includegraphics{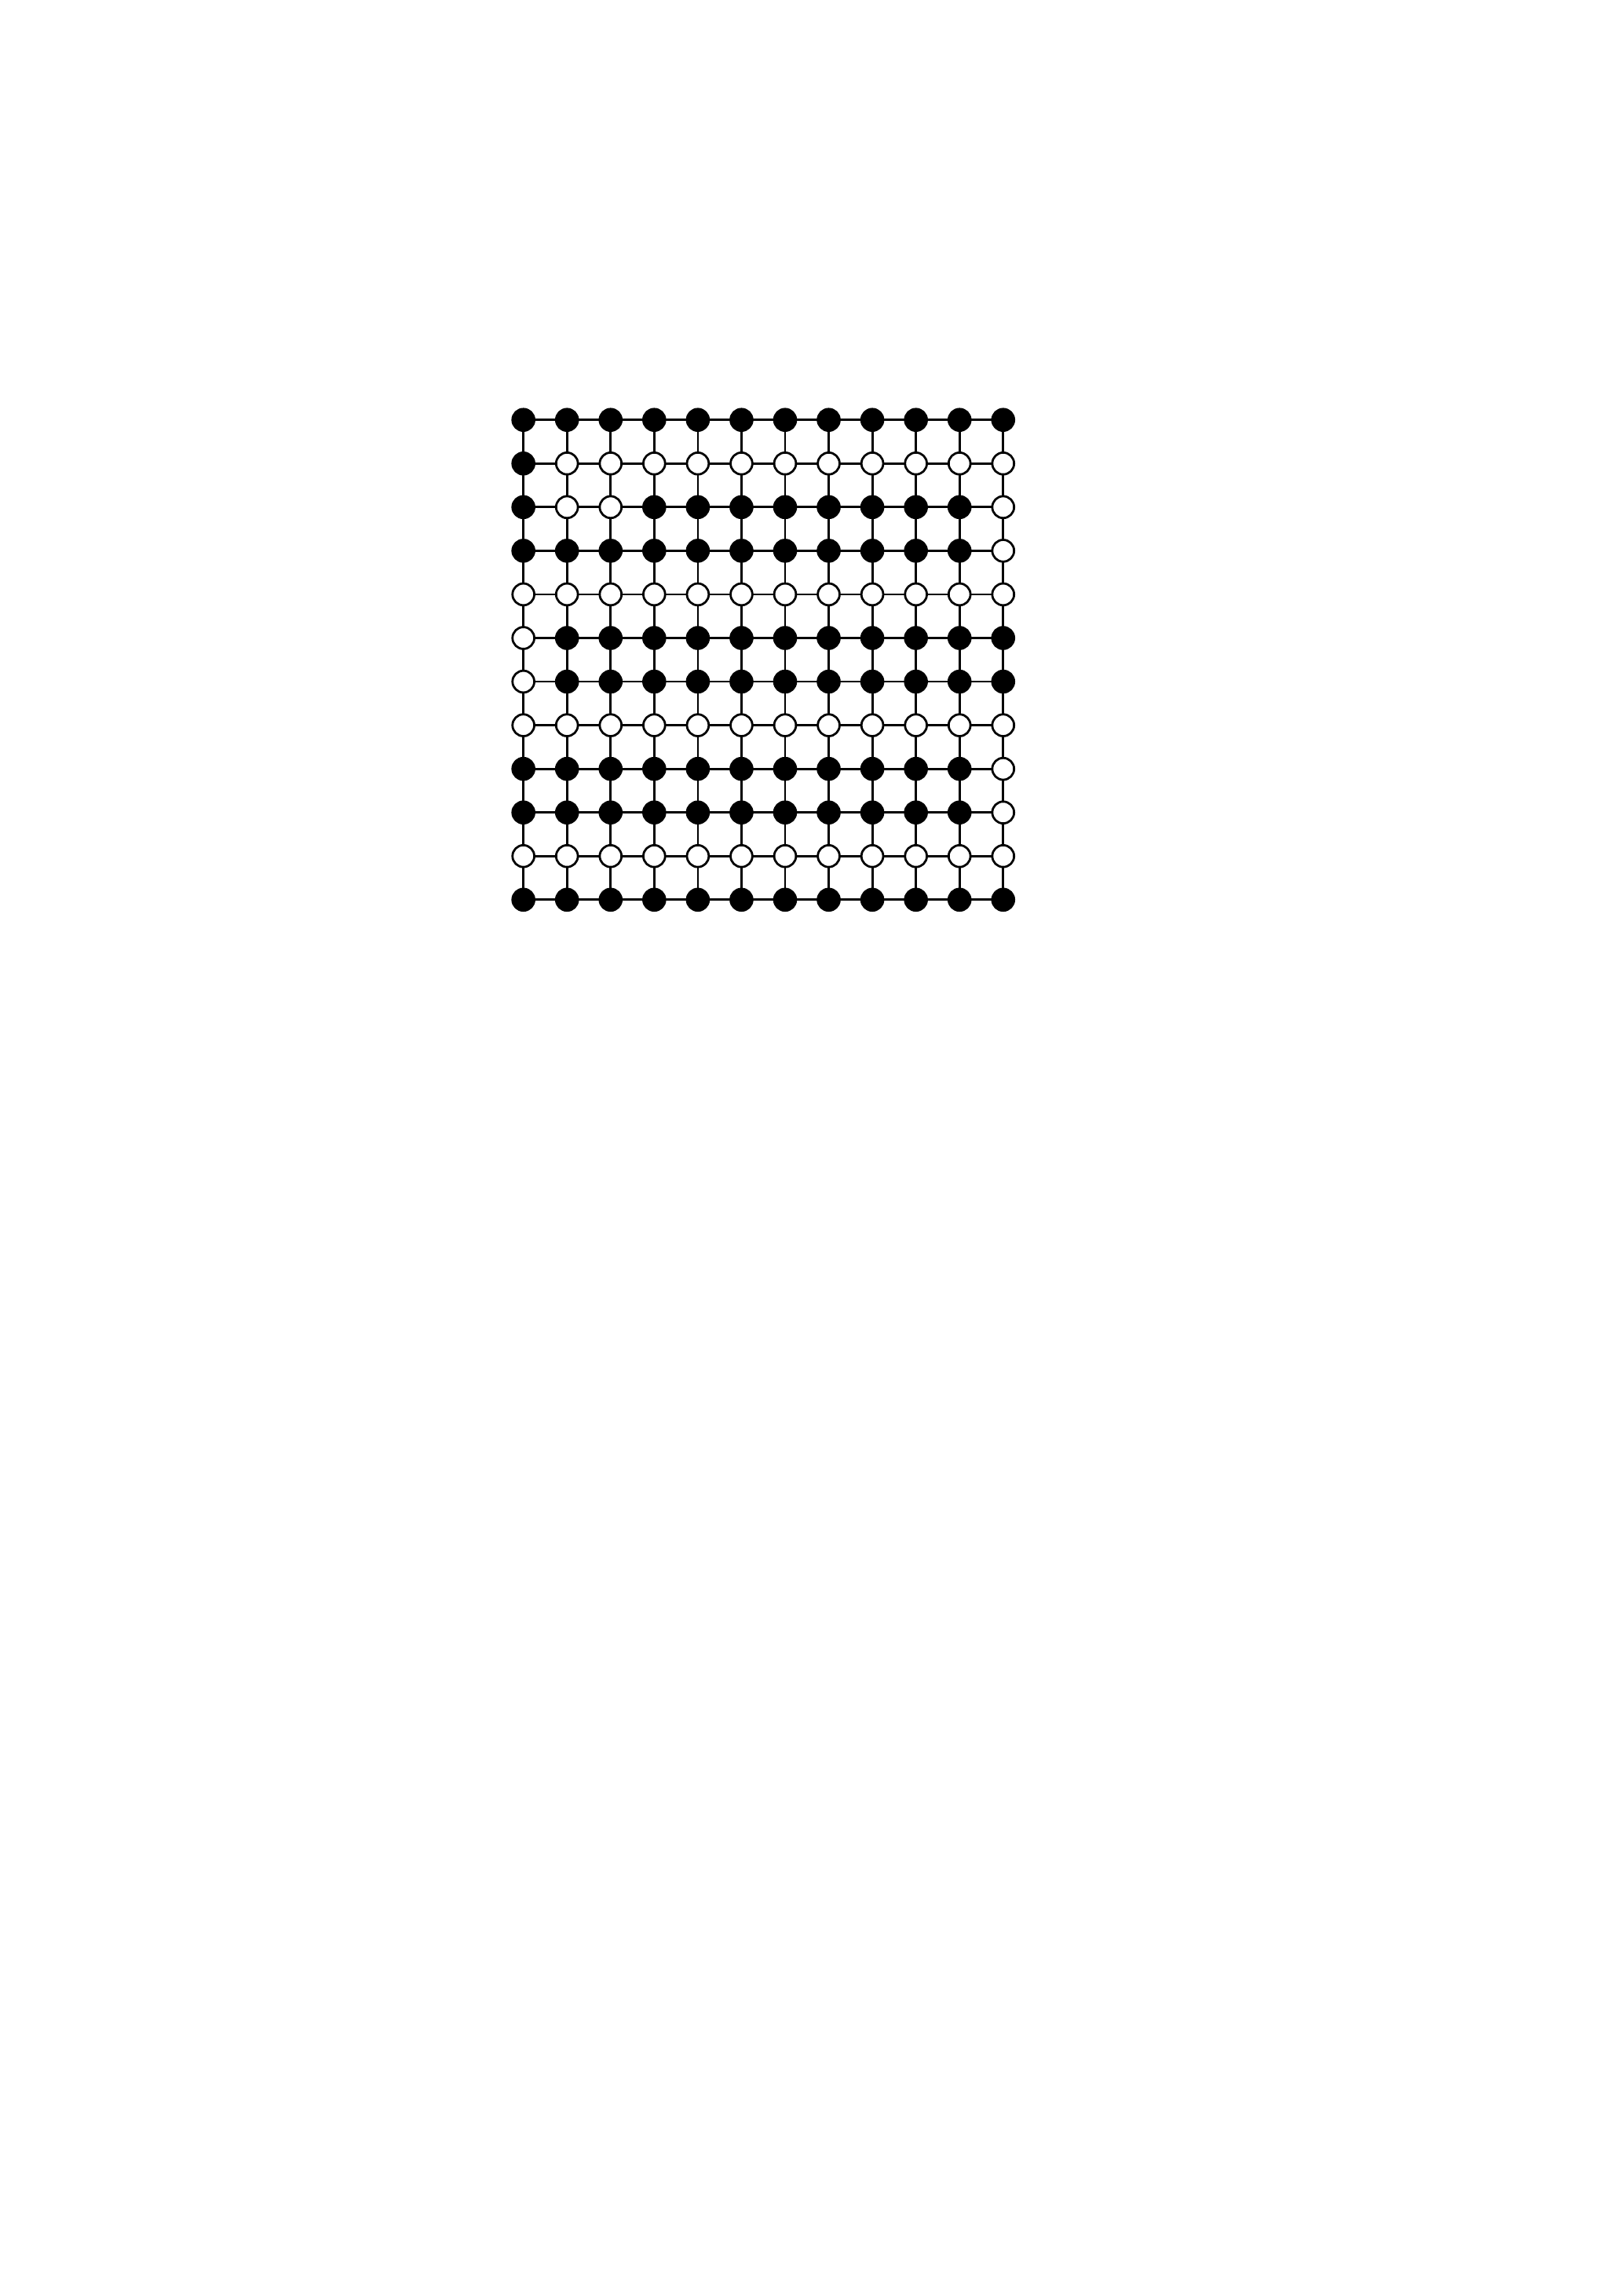}
\caption{A two-dimensional grid with an initial opinion assignment that
\stabil s only after $\BigOmega{n}$ steps.}
\label{fig:example-grid}
\end{figure}

One might intuitively think that an expression based on the diameter of the
underlying network might be a suitable upper bound for the \dtime.
However, the following example of a two-dimensional grid shows that this is not
true. We are given a two-dimensional grid $G$ of size $|V| = \sqrt{n} \times
\sqrt{n}$. Clearly, the diameter of this graph is $2\cdot\sqrt{n}$. However, by
laying a winding \emph{serpentine} path of white nodes in an entirely black
grid as initial opinion assignment $f$ we can force the process to require a
\dtime of $\ctime(G, f) = \BigOmega{n} \gg \operatorname{diam}(G) =
\BigO{\sqrt{n}}$. This example is shown in \autoref{fig:example-grid}.

\subsection{The Circle}

\begin{figure}[h]
\centering
\begin{subfigure}{0.45\textwidth} \centering
\includegraphics{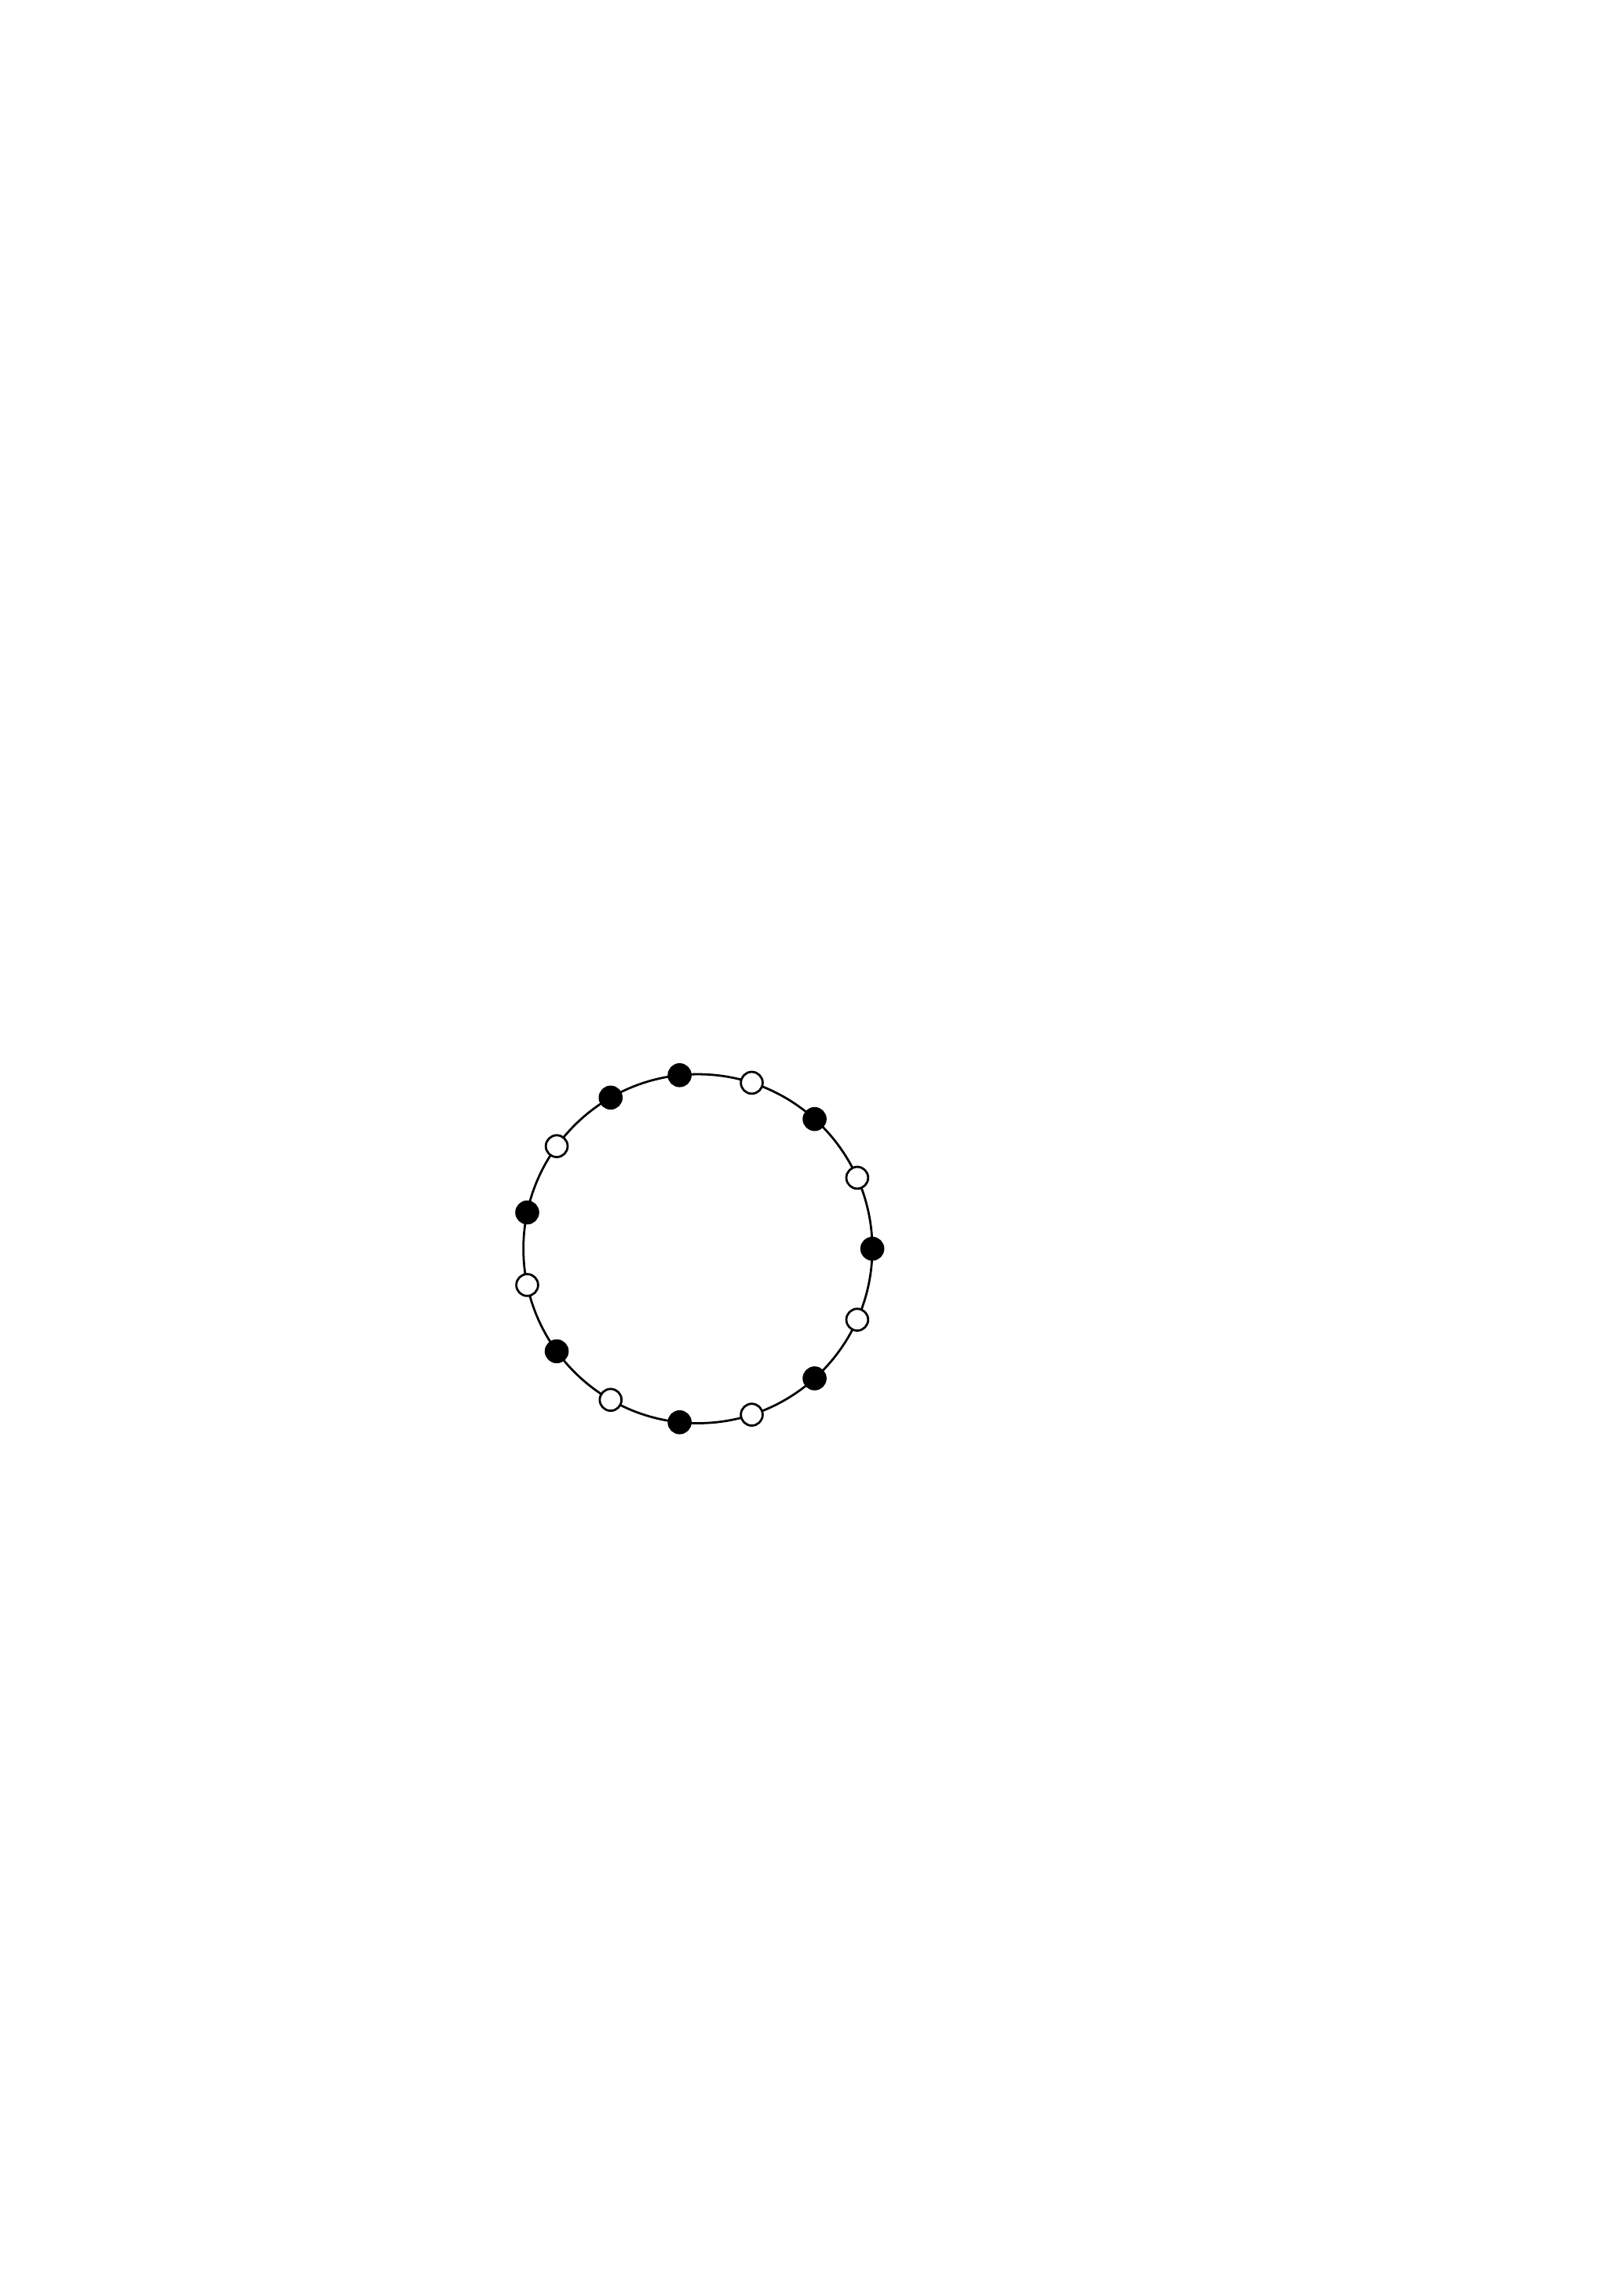}
\caption{circle with \dtime $|E|/2 \pm \BigO{1}$}
\label{fig:example-circle-1}
\end{subfigure}
\begin{subfigure}{0.45\textwidth} \centering
\includegraphics{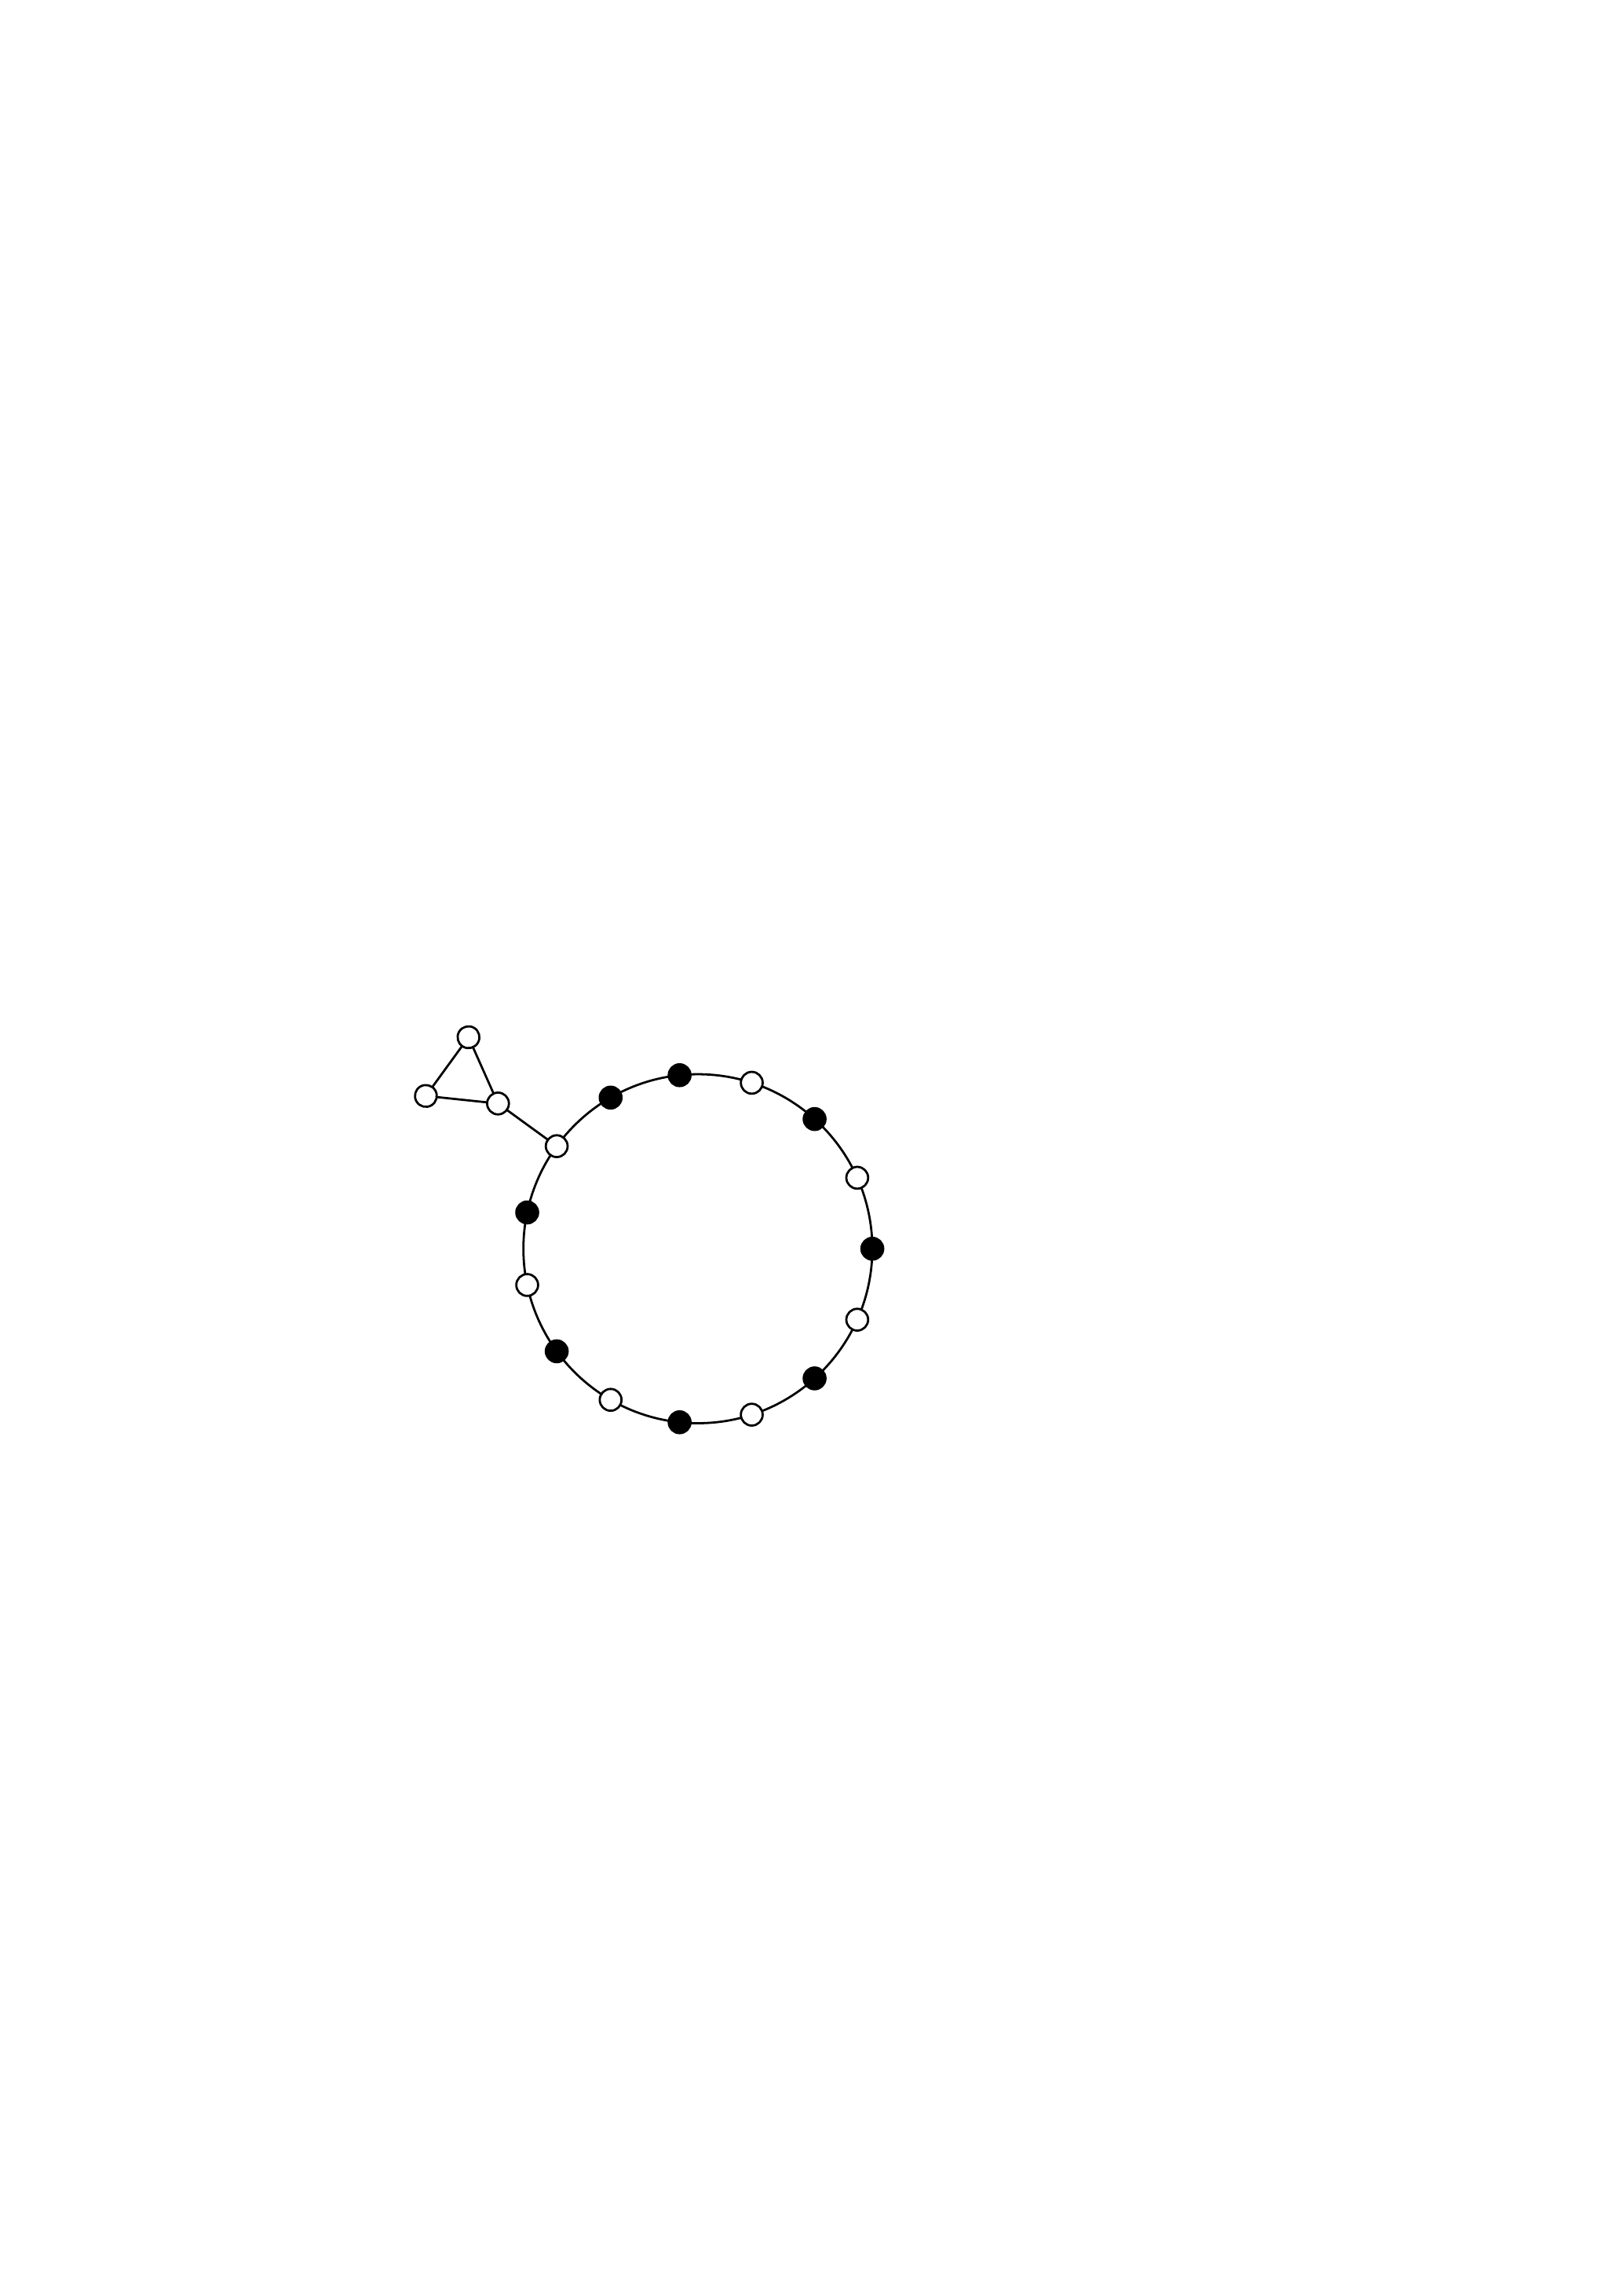}
\caption{circle with gadget, \dtime $|E| \pm \BigO{1}$}
\label{fig:example-circle-2}
\end{subfigure}

\caption{The circle has a \dtime of at most $|E|/2$. However, adding a small
gadget almost doubles the \dtime.}
\label{fig:example-circle}
\end{figure}

In \autoref{sect:main-result} we analyzed the tightness of
\autoref{thm:E_upper} for several graph classes. This bound is reached up to
one in a path graph where each pair of consecutive nodes has alternating
opinions except for the last two nodes, which share the same opinion.
Interestingly, when changing the graph from a path to a circle, the \dtime
 drops by a factor of two. Indeed, it is not hard to prove that the longest
\dtime for the circle is achieved by the initial opinion assignment
in which black and whites nodes alternate, except for a single pair of adjacent
black nodes. An example is shown in \autoref{fig:example-circle-1}. However,
adding only a small gadget to the circle again pushes the \dtime up
to the same number of steps as required for the path (up to an additive
constant for the gadgets). This gadget is shown in
\autoref{fig:example-circle-2}.
